# Supplementary material for: Finite-source magnification residuals from a cNFW-inspired perturbation of an effective spinning black hole binary lens
Source: arXiv:2607.23300 source file (2026-09-27)
Supplement: Supplementary file 1 [file caustic_dm_supplement.tex]

\documentclass[10pt]{article}

\usepackage[T1]{fontenc}
\usepackage{lmodern}
\usepackage[a4paper,margin=1.8cm]{geometry}
\usepackage{amsmath,amssymb}
\usepackage{booktabs}
\usepackage{graphicx}
\usepackage{float}
\usepackage[hidelinks]{hyperref}
\usepackage{microtype}

\setlength{\textfloatsep}{8pt plus 2pt minus 2pt}
\setlength{\floatsep}{8pt plus 2pt minus 2pt}
\setlength{\intextsep}{8pt plus 2pt minus 2pt}
\raggedbottom

\title{Supplementary Material for\\
\textit{Dark matter imprints on a caustic encounter in an effective spinning black hole binary lens}}
\author{Mohsen Fathi}
\date{}

\begin{document}
\maketitle

\section{Why this supplement is included}

The Letter asks one specific question.  If a spinning vacuum binary is fitted
to an effective binary with a cored Navarro--Frenk--White (cNFW) correction,
does any numerically resolved caustic difference remain?  The calculation
uses a quasi-stationary effective lens map.  It is not an exact binary Kerr
spacetime and it is not a numerical-relativity ray trace.  The cNFW factor is
used only as a phenomenological radial correction inspired by
Ref.~\cite{Senjaya2026}.  An empirical halo profile does not, by itself,
define a self-consistent relativistic matter solution \cite{Bolokhov2026}.

This supplement gives the model settings, the wider vacuum comparison, the
spin-reversal and resolution checks, and a check of every rising
half-response crossing.  Its purpose is simple: to show what has been tested
and what is still outside the present model.

\section{Model settings and trajectory}

Table~\ref{tab:parameters} lists the cNFW benchmark and the best vacuum model.
All quantities are given in dimensionless effective lens units.

\begin{table}[H]
\centering
\caption{Benchmark parameters.  A dash means that the parameter is absent in
the vacuum model.}
\label{tab:parameters}
\begin{tabular}{lcc}
\toprule
Quantity & cNFW benchmark & best vacuum \\
\midrule
Mass ratio $q=m_2/m_1$ & 1.000 & 1.000 \\
Binary separation $d$ & 0.340 & 0.340 \\
Lens scale $A$ & 0.0320 & 0.0326 \\
Softening $\epsilon$ & 0.022 & 0.022 \\
Common spin $\chi$ & 0.85 & 0.84 \\
Projected spin angle $\gamma$ & $25^\circ$ & $25^\circ$ \\
Spin coefficient $\kappa_J$ & 0.18 & 0.18 \\
Halo strength $\eta$ & 0.0025 & 0 \\
Core scale $\lambda_{\rm c}$ & 10 & -- \\
Halo gain $g_{\rm h}$ & 6 & 0 \\
Radial mapping scale $R_\star$ & 40 & -- \\
Source radius $R_{\rm s}$ & 0.030 & 0.030 \\
\bottomrule
\end{tabular}
\end{table}

We set $m_1+m_2=1$, with $m_1=1/(1+q)$ and $m_2=q/(1+q)$.  In the
unequal-mass vacuum trials, the two components move around their common
centre:
\begin{equation}
\boldsymbol{\theta}_1(\Phi)
=d m_2(\cos2\pi\Phi,\sin2\pi\Phi),
\qquad
\boldsymbol{\theta}_2(\Phi)
=-d m_1(\cos2\pi\Phi,\sin2\pi\Phi).
\end{equation}
For $q=1$, these positions reduce to $\pm d/2$.  The source centre follows
\begin{equation}
\boldsymbol{\beta}_{\rm s}(\Phi)
=\bigl(0.23\cos\psi,0.085\sin2\psi\bigr),
\qquad
\psi=2\pi\Phi+0.35,
\end{equation}
with $R_{\rm s}=0.030$.  The Jacobian is sampled over
$\theta_x\in[-0.72,0.72]$ and $\theta_y\in[-0.47,0.47]$.

The finite-source response is
\begin{equation}
\mathcal C(\Phi)=
\left[1+\exp\left(
\frac{d_{\min}(\Phi)-R_{\rm s}}{0.18R_{\rm s}}
\right)\right]^{-1},
\end{equation}
where $d_{\min}$ is the shortest distance between the source centre and the
extracted caustic.  This response is a smooth clock for the encounter.  It is
not an observed flux.

\section{How the vacuum comparison is made}

The phase offset is fitted over the complete orbit.  We first minimize
\begin{equation}
\mathcal R_{\rm orb}
=
\left\langle
[\mathcal C_{\rm cNFW}(\Phi)
-\mathcal C_{\rm vac}(\Phi+\delta\Phi)]^2
\right\rangle_{\rm orb}^{1/2}
\end{equation}
over the tested vacuum parameters.  We then measure the local residual
$\mathcal R_{\mathcal W}$ in the window
$|\Phi-\Phi_{\rm mid}|\leq0.115$, without fitting the phase again.
Here $\Phi_{\rm mid}$ is the midpoint of the cNFW crossing and the globally
aligned vacuum crossing.  The local rms can therefore be smaller than
$\mathcal R_{\rm orb}$ when the selected window leaves out larger residual
features elsewhere in the orbit; no second fit is made inside the window.

The first local grid uses
\begin{align}
A&\in\{0.0325,0.0326,0.0327\},\\
\chi&\in\{0.80,0.84,0.88\},\\
d&\in\{0.335,0.340,0.345\}.
\end{align}
Figure~\ref{fig:library} shows this grid.  Its overall minimum is at
$A=0.0326$, $\chi=0.84$, and $d=0.340$.

\begin{figure}[H]
\centering
\includegraphics[width=0.96\textwidth]{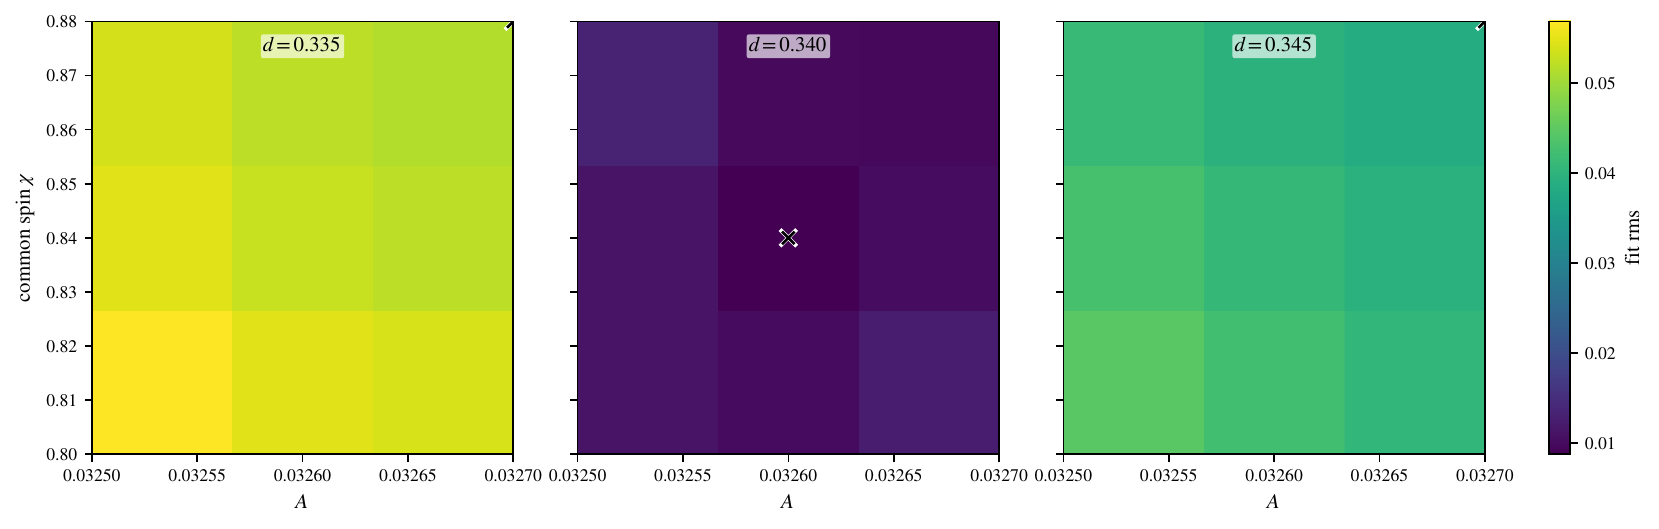}
\caption{The first local vacuum grid.  Each panel fixes the separation and
shows the phase-profiled rms residual over lens scale and common spin.  The
cross marks the minimum in each panel.}
\label{fig:library}
\end{figure}

We then made the comparison wider.  The coarse scan used
$q\in\{0.8,1.0,1.2\}$ and
$\gamma\in\{15^\circ,25^\circ,35^\circ\}$.  At every point we also profiled
$A$, the common spin $\chi$, the separation $d$, and the phase offset.  A
second scan used the smaller ranges
$q\in\{0.9,1.0,1.1\}$ and
$\gamma\in\{20^\circ,25^\circ,30^\circ\}$ around the best point.
Figure~\ref{fig:expanded} shows the coarse scan.  Its minimum lies inside both
tested ranges, at $q=1$ and $\gamma=25^\circ$.

\begin{figure}[H]
\centering
\includegraphics[width=0.62\textwidth]{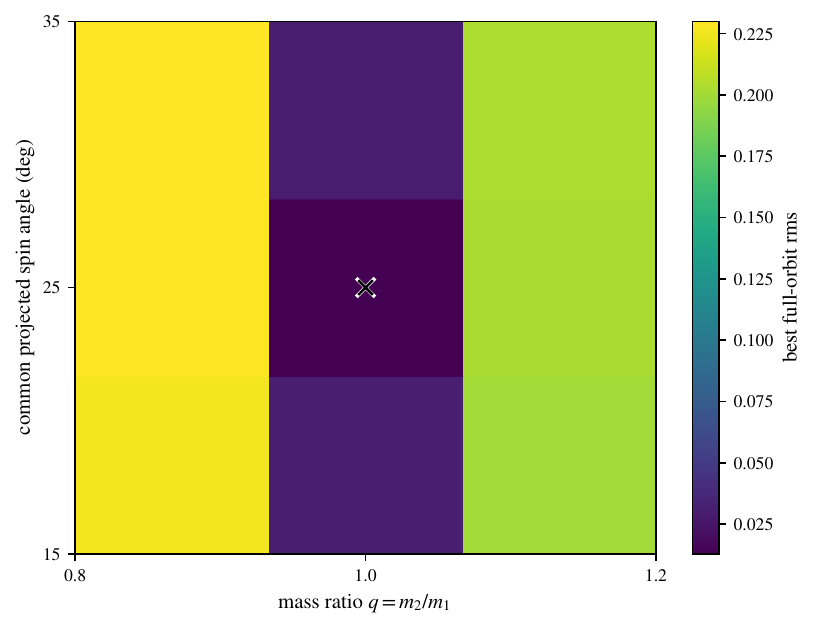}
\caption{Expanded coarse vacuum scan.  Each cell shows the lowest full-orbit
rms after fitting $A$, common $\chi$, $d$, and phase at fixed mass ratio and
common projected spin angle.  The cross marks the coarse minimum.}
\label{fig:expanded}
\end{figure}

The ten best candidates from the coarse and refined scans were recalculated
with 240 phases and a $170\times110$ contour grid.  All ten had $q=1$ and
$\gamma=25^\circ$.  We then checked nearby unequal component spins and
unequal projected directions around this best point.  Table~\ref{tab:expanded}
shows the most useful cases.  All rows use $d=0.340$.

\begin{table}[H]
\centering
\small
\caption{High-resolution checks around the best vacuum model.  Angles are in
degrees.}
\label{tab:expanded}
\begin{tabular}{lcccccc}
\toprule
Case & $q$ & $(\chi_1,\chi_2)$ & $(\gamma_1,\gamma_2)$ & $A$ & $\mathcal R_{\rm orb}$ & $\mathcal R_{\mathcal W}$ \\
\midrule
Best common & 1.0 & $(0.84,0.84)$ & $(25,25)$ & 0.0326 & 0.01540 & 0.01341 \\
Spin split & 1.0 & $(0.80,0.88)$ & $(25,25)$ & 0.0326 & 0.01732 & 0.01426 \\
Spin split & 1.0 & $(0.88,0.80)$ & $(25,25)$ & 0.0326 & 0.02013 & 0.01212 \\
Angle split & 1.0 & $(0.84,0.84)$ & $(20,30)$ & 0.0326 & 0.01986 & 0.01539 \\
Angle split & 1.0 & $(0.84,0.84)$ & $(30,20)$ & 0.0326 & 0.01860 & 0.01590 \\
\bottomrule
\end{tabular}
\end{table}

The equal-mass, common-spin model gives the smallest full-orbit residual.
Some split-spin cases give a slightly smaller residual inside the selected
window, but their full-orbit fit is worse.  This is why the model and phase
are chosen from the whole orbit rather than from one local event.

This parameter check is still finite.  It does not cover arbitrary
three-dimensional spin vectors.  It also does not add an independent orbital
inclination, because inclination is not a separate variable in the projected
two-dimensional map used here.

\section{Basic code checks}

Setting $\chi_1=\chi_2=0$ gives the mass-only map to machine precision.
Setting $\eta=g_{\rm h}=0$ gives the spinning vacuum map.  At the level of the
lens map, the spin term is odd under simultaneous spin reversal to
$2.22\times10^{-16}$.

A centroid measured from extracted caustic contours is a nonlinear and
grid-dependent quantity.  To define the check, let
$\boldsymbol c_{+}$, $\boldsymbol c_{-}$, and $\boldsymbol c_{0}$ be the
caustic centroids for positive, negative, and zero spin.  We use the
dimensionless quantity
\begin{equation}
D_{\rm c}
=
\frac{\left\|\boldsymbol c_{+}+\boldsymbol c_{-}-2\boldsymbol c_{0}\right\|}
{\max\!\left(\left\|\boldsymbol c_{+}-\boldsymbol c_{0}\right\|,
\left\|\boldsymbol c_{-}-\boldsymbol c_{0}\right\|,10^{-14}\right)}.
\end{equation}
It measures the departure of the extracted centroid from a linear odd
response under spin reversal.  Table~\ref{tab:reversal} shows that
$D_{\rm c}$ falls rapidly as the contour grid is refined.  We use it only as
an extraction and convergence check, not as a failed exact symmetry test.

\begin{table}[H]
\centering
\caption{Spin-reversal checks at orbital phase $\Phi=0.25$.  The centroid
quantity $D_{\rm c}$ is dimensionless.}
\label{tab:reversal}
\begin{tabular}{lcc}
\toprule
Contour grid & map-level oddness error & $D_{\rm c}$ \\
\midrule
$240\times154$ & $2.22\times10^{-16}$ & 0.33531 \\
$320\times205$ & $2.22\times10^{-16}$ & 0.01606 \\
$480\times308$ & $2.22\times10^{-16}$ & 0.00261 \\
\bottomrule
\end{tabular}
\end{table}

\section{Resolution check}

The main calculation uses 240 orbital phases and a $170\times110$ contour
grid.  We compare it with a nearby calculation using 200 phases and a
$160\times104$ grid.  Table~\ref{tab:resolution} lists the values, while
Fig.~\ref{fig:resolution} compares the response curves and local residual.

\begin{table}[H]
\centering
\caption{Resolution comparison for the selected encounter.  The aligned
crossing is measured after the full-orbit phase fit.}
\label{tab:resolution}
\begin{tabular}{lcc}
\toprule
Quantity & $240$, $170\times110$ & $200$, $160\times104$ \\
\midrule
cNFW crossing & 0.079412 & 0.079023 \\
Raw vacuum crossing & 0.077405 & 0.076832 \\
Aligned vacuum crossing & 0.077905 & 0.077207 \\
Aligned crossing shift & 0.001507 & 0.001816 \\
Window rms $\mathcal R_{\mathcal W}$ & 0.013410 & 0.014963 \\
Window $\max|\Delta\mathcal C|$ & 0.040203 & 0.040238 \\
Full-orbit rms & 0.015397 & 0.012957 \\
\bottomrule
\end{tabular}
\end{table}

\begin{figure}[H]
\centering
\includegraphics[width=0.88\textwidth]{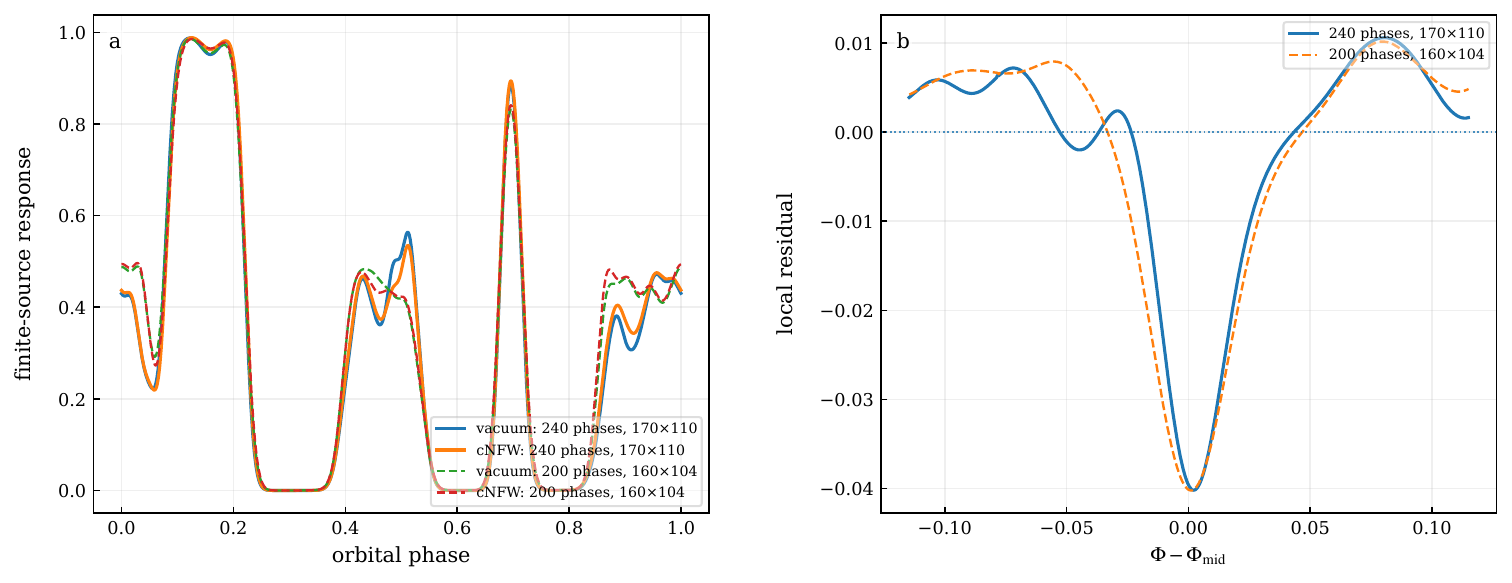}
\caption{Resolution comparison.  Left: the vacuum and cNFW responses at the
two numerical settings.  Right: the globally aligned residual in the
selected encounter window.}
\label{fig:resolution}
\end{figure}

The window rms changes by $1.55\times10^{-3}$, the maximum local residual by
less than $4\times10^{-5}$, and the aligned crossing shift by
$3.09\times10^{-4}$.  The full-orbit rms is slightly smaller on the coarser
grid, so this two-level comparison is not a formal convergence-order test.
It is used only to check that the quoted local features do not disappear under
a nearby change of resolution.

\section{Check of all rising crossings}

The response has three rising half-response crossings.  We use the event near
$\Phi\simeq0.08$ because it can be followed in both models and at both
resolutions.  It was not chosen because it gives the largest shift.
Table~\ref{tab:crossings} lists all three events after the single global phase
fit, and Fig.~\ref{fig:crossings} shows them over the full orbit.

\begin{table}[H]
\centering
\small
\caption{All rising half-response crossings.  The local rms and maximum are
measured in a window of half-width $0.04$ around each cNFW crossing.}
\label{tab:crossings}
\begin{tabular}{crrrrr}
\toprule
Event & $\Phi_{\rm cNFW}$ & $\Phi_{\rm vac,al}$ & $\Delta\Phi_{\rm al}$ & local rms & local max \\
\midrule
1 & 0.079412 & 0.077905 & $+0.001507$ & 0.02126 & 0.04020 \\
2 & 0.503396 & 0.488011 & $+0.015385$ & 0.02877 & 0.05259 \\
3 & 0.676630 & 0.677581 & $-0.000950$ & 0.01649 & 0.03221 \\
\bottomrule
\end{tabular}
\end{table}

\begin{figure}[H]
\centering
\includegraphics[width=0.64\textwidth]{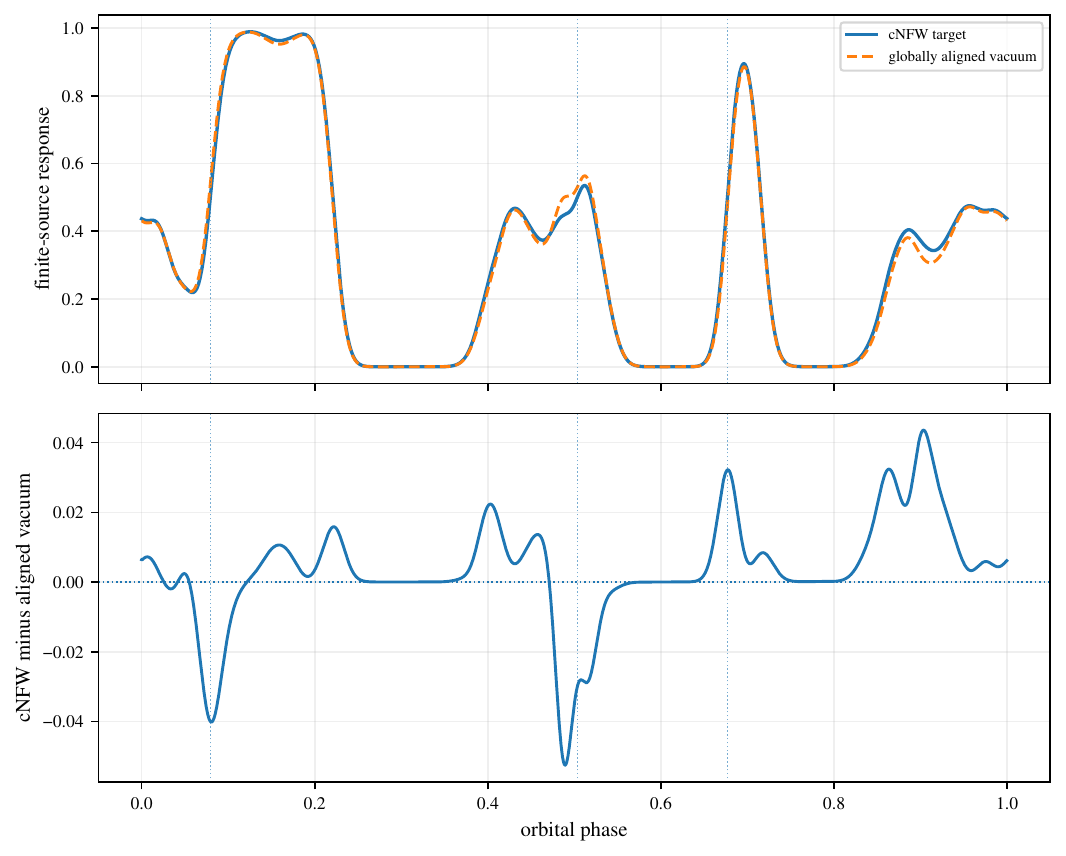}
\caption{Full-orbit crossing check.  Top: the cNFW response and the globally
aligned vacuum response.  Bottom: their residual.  The dotted vertical lines
mark all rising cNFW half-response crossings.}
\label{fig:crossings}
\end{figure}

The event used in the Letter is not the strongest event in either crossing
shift or local rms.  Listing all three events makes the selection rule clear
and avoids treating the benchmark as a look-elsewhere-optimised signal.

\section{Nearby exploratory cases}

We also changed the halo strength, source radius, and separation while
keeping the same refined vacuum reference.  The vacuum model was not fitted
again for each row.  The values in Table~\ref{tab:variations} are therefore
simple diagnostics, not exclusion significances.

\begin{table}[H]
\centering
\caption{Exploratory fixed-reference variations.  These values use the
earlier fixed-reference crossing convention and should not be compared
directly with the globally aligned shifts in Tables~\ref{tab:resolution} and
\ref{tab:crossings}.}
\label{tab:variations}
\begin{tabular}{lrrr}
\toprule
Case & crossing shift & rms & $\max|\Delta\mathcal C|$ \\
\midrule
$\eta=0.001$ & $+0.000235$ & 0.02038 & 0.08614 \\
$\eta=0.0025$ & $+0.002435$ & 0.01215 & 0.04305 \\
$R_{\rm s}=0.024$ & $+0.009023$ & 0.08092 & 0.20846 \\
$R_{\rm s}=0.036$ & $-0.007295$ & 0.06976 & 0.14740 \\
$d=0.306$ & $+0.02051$ & 0.17254 & 0.44369 \\
$d=0.374$ & $-0.05091$ & 0.18333 & 0.81438 \\
\bottomrule
\end{tabular}
\end{table}

These cases show that the sign and size of a crossing shift are not universal.
This is why the Letter makes only a local benchmark statement.

\section{Companion movie}

Movie~S1 follows one complete orbit.  The left panel shows the best-fit
spinning vacuum image, and the middle panel shows the cNFW image at the same
phase.  Their small source-plane insets show the local caustic and the finite
source.  The right panel follows the two finite-source responses.  The full
images look similar because the vacuum model was fitted to imitate the cNFW
case.  The remaining difference is easier to see in the response curves and
crossing phases.

\end{document}
